# Supplementary material for: Regression Filtration with Resetting to Provide Exponential Convergence of MRAC for Plants with Jump Change of Unknown Parameters
Source: arXiv:2102.10359 ancillary file (2022-10-10)
Supplement: Supplementary file 1 [file supp.pdf]

# Supplement to “Regression Filtration with Resetting to Provide Exponential Convergence of MRAC for Plants with Jump Change of Unknown Parameters” in IEEE-TAC

Anton Glushchenko, *Memner, IEEE*, Vladislav Petrov, and Konstantin Lastochkin

## Abstract

This article is supplementary material for the technical note “Regression Filtration with Resetting to Provide Exponential Convergence of MRAC for Plants with Jump Change of Unknown Parameters” in IEEE Transactions on Automatic Control by the same authors. It gives proofs of the lemmas, propositions and theorems, presents some additional simulation results and is being referred in appropriate places in the note.

## I. PROOF OF LEMMA 1 IN THE MANUSCRIPT

**Lemma 1.** Let  $k > 0$  be sufficiently large, then the filtered value  $\Delta_f(t) \in \mathbb{R}^m$  of uncertainty  $\Delta(t)$  is evaluated as follows:

$$\Delta_f(t) = B^\dagger \left( e_{ref}(t) - k e_f(t) - e^{-k(t-t_r^+)} e_{ref}(t_r^+) - A_{ref} e_f(t) + B u_{adf}(t) \right) = \Theta^T(t) \Phi_f(x(t)). \quad (S1)$$

*Proof.* The equation (10) in the manuscript is substituted into the solution of the first equation of (11) in the manuscript to obtain:

$$\begin{aligned} \mu_f(t) &= e^{-k(t-t_r^+)} \mu_f(t_r^+) + e^{-kt} \int_{t_r^+}^t e^{k\tau} \dot{e}_{ref}(\tau) d\tau = e^{-k(t-t_r^+)} \mu_f(t_r^+) + \\ &\quad + e^{-kt} \int_{t_r^+}^t e^{k\tau} \left( A_{ref} e_{ref}(\tau) + B \tilde{\Theta}^T(\tau) \Phi(x(\tau)) \right) d\tau = \\ &= e^{-k(t-t_r^+)} \mu_f(t_r^+) + A_{ref} e^{-kt} \int_{t_r^+}^t e^{k\tau} e_{ref}(\tau) d\tau + B e^{-kt} \int_{t_r^+}^t e^{k\tau} \Theta^T(\tau) \Phi(x(\tau)) d\tau - \\ &\quad - B e^{-kt} \int_{t_r^+}^t e^{k\tau} \hat{\Theta}^T(\tau) \Phi(x(\tau)) d\tau. \end{aligned} \quad (S2)$$

The solutions of the second equation of (11) in the manuscript and the first equation of (12) in the manuscript are written as:

$$\begin{aligned} e_f(t) &= e^{-k(t-t_r^+)} e_f(t_r^+) + e^{-kt} \int_{t_r^+}^t e^{k\tau} e_{ref}(\tau) d\tau, \\ u_{adf}(t) &= e^{-k(t-t_r^+)} u_{adf}(t_r^+) + e^{-kt} \int_{t_r^+}^t e^{k\tau} \hat{\Theta}^T(\tau) \Phi(x(\tau)) d\tau. \end{aligned} \quad (S3)$$

Then the equation (S2) is rewritten as:

$$\begin{aligned} \mu_f(t) &= e^{-k(t-t_r^+)} \mu_f(t_r^+) - A_{ref} e^{-k(t-t_r^+)} e_f(t_r^+) + B e^{-k(t-t_r^+)} u_{adf}(t_r^+) + A_{ref} e_f(t) + \\ &\quad + B e^{-kt} \int_{t_r^+}^t e^{k\tau} \Theta^T(\tau) \Phi(x(\tau)) d\tau - B u_{adf}(t) \end{aligned} \quad (S4)$$

Let an axillary equation be introduced:

$$\mu_{fd}(t) = A_{ref} e_f(t) - B u_{adf}(t). \quad (S5)$$

Then the filtered parameter uncertainty  $\Delta_f(t) \in \mathbb{R}^m$  of the plant can be found on the basis of (S4) and (S5):

$$\begin{aligned} \Delta_f(t) &= B^\dagger (\mu_f(t) - \mu_{fd}(t)) = \\ &= B^\dagger \left( e^{-k(t-t_r^+)} \mu_f(t_r^+) - A_{ref} e^{-k(t-t_r^+)} e_f(t_r^+) + B e^{-k(t-t_r^+)} u_{adf}(t_r^+) + A_{ref} e_f(t) + \right. \\ &\quad \left. + B e^{-kt} \int_{t_r^+}^t e^{k\tau} \Theta^T(\tau) \Phi(x(\tau)) d\tau - B u_{adf}(t) - A_{ref} e_f(t) + B u_{adf}(t) \right) = \\ &= B^\dagger \left( e^{-k(t-t_r^+)} \mu_f(t_r^+) - A_{ref} e^{-k(t-t_r^+)} e_f(t_r^+) + B e^{-k(t-t_r^+)} u_{adf}(t_r^+) + B e^{-kt} \int_{t_r^+}^t e^{k\tau} \Theta^T(\tau) \Phi(x(\tau)) d\tau \right). \end{aligned} \quad (S6)$$

Research was partly financially supported by Grants Council of the President of the Russian Federation (project MD-1787.2022.4).

A. I. Glushchenko is with V.A. Trapeznikov Institute of Control Sciences RAS, Moscow, Russia (phone: +79102266946; e-mail: aiglush@ipu.ru).

V. A. Petrov is with Stary Oskol technological institute (branch) NUST “MISIS”, Stary Oskol, Russia (e-mail: petrov.va@misis.ru).

K. A. Lastochkin is with V.A. Trapeznikov Institute of Control Sciences RAS, Moscow, Russia (e-mail: lastconst@ipu.ru).

Considering the initial conditions from (11) and (12) in the manuscript, the equation (S6) is rewritten as:

$$\Delta_f(t) = B^\dagger \left( B e^{-kt} \int_{t_r^+}^t e^{k\tau} \Theta^T(\tau) \Phi(x(\tau)) d\tau \right) = e^{-kt} \int_{t_r^+}^t e^{k\tau} \Theta^T(\tau) \Phi(x(\tau)) d\tau. \quad (S7)$$

As the commutativity property with respect to  $\Theta^T(t)$  does not hold for the integral in (S7), then the right-hand side of (S7) is added and subtracted with  $\Theta^T(t) \Phi_f(x(t))$ :

$$\Delta_f(t) = \underbrace{\Theta^T(t) \Phi_f(x(t)) + e^{-kt} \int_{t_r^+}^t e^{k\tau} \Theta^T(\tau) \Phi(x(\tau)) d\tau - \Theta^T(t) \Phi_f(x(t))}_{\epsilon(t)}. \quad (S8)$$

The error  $\epsilon$  is represented in the state space:

$$\begin{aligned} \epsilon(t) &= \chi(t) - \Theta^T(t) \Phi_f(x(t)), \quad \epsilon(t_r^+) = 0_m, \\ \dot{\chi}(t) &= -k\chi(t) + \Theta^T(t) \Phi(x(t)), \quad \chi(t_r^+) = 0_m. \end{aligned} \quad (S9)$$

Taking into consideration (4), (12) in the manuscript and (S9), the error  $\epsilon$  is differentiated:

$$\begin{aligned} \dot{\epsilon}(t) &= \dot{\chi}(t) - \dot{\Theta}^T(t) \Phi_f(x(t)) - \Theta^T(t) \dot{\Phi}_f(x(t)) = \\ &= -k\chi(t) + \Theta^T(t) \Phi(x(t)) - \dot{\Theta}^T(t) \Phi_f(x(t)) - \Theta^T(t) [-k\Phi_f(x(t)) + \Phi(x(t))] = \\ &= -k[\chi(t) - \Theta^T(t) \Phi_f(x(t))] - \dot{\Theta}^T(t) \Phi_f(x(t)) = -k\epsilon(t) - \dot{\Theta}^T(t) \Phi_f(x(t)) = -k\epsilon(t) - \sum_j \theta_j^T \delta(t - t_j) \Phi_f(x(t_j)). \end{aligned} \quad (S10)$$

According to the properties of the delta-function, the solution of (S10) is written as:

$$\begin{aligned} \epsilon(t) &= e^{-k(t-t_r^+)} \epsilon(t_r^+) - e^{-kt} \int_{t_r^+}^t e^{k\tau} \sum_j \theta_j^T \delta(\tau - t_j) \Phi_f(x(\tau)) d\tau = \\ &= e^{-k(t-t_r^+)} \epsilon(t_r^+) - e^{-kt} \sum_j e^{kt_j} \theta_j^T h(t - t_j) \Phi_f(x(t_j)). \end{aligned} \quad (S11)$$

As  $\epsilon(t_r^+) = 0_m$ , then the following piecewise definition is obtained on the basis of (S11):

$$\epsilon(t) = \begin{cases} 0_m, & \forall t \in [t_r^+; t_j) \\ -e^{-kt} \sum_j e^{kt_j} \theta_j^T h(t - t_j) \Phi_f(x(t_j)), & \forall t \geq t_j \end{cases}. \quad (S12)$$

or, if we consider the definition of  $t_r^+$ , then:

$$\epsilon(t) = \begin{cases} 0_m, & \forall t \in [t_k; t_j) \\ -e^{-kt} \sum_j e^{kt_j} \theta_j^T h(t - t_j) \Phi_f(x(t_j)), & \forall t \in [t_j; t_{k+1}) \end{cases}. \quad (S13)$$

Whence it follows that, if  $k > 0$  is chosen to be sufficiently large, then the equation  $\epsilon(t) = o(\Theta^T(t) \Phi_f(x(t)))$  holds almost everywhere. As a result, the equation (S8) is rewritten without  $\epsilon(t)$ :

$$\Delta_f(t) = \Theta^T(t) \Phi_f(x(t)). \quad (S14)$$

Then  $\mu_f(t)$  is calculated using the measurable signals only, i.e. without knowledge about  $\dot{e}_{ref}(t)$ . The value of  $\int_{t_r^+}^t e^{k\tau} \dot{e}_{ref}(\tau) d\tau$  from (S2) is found using the integration by parts:

$$\begin{aligned} \int_{t_r^+}^t e^{k\tau} \dot{e}_{ref}(\tau) d\tau &\equiv \left[ u = e^{k\tau}; du = k e^{k\tau} d\tau \right]_{dv = \dot{e}_{ref}(\tau) d\tau; v = e_{ref}(\tau)} = uv|_{t_r^+}^t - \int_{t_r^+}^t v du = e^{kt} e_{ref}(t) - e^{kt_r^+} e_{ref}(t_r^+) - k \int_{t_r^+}^t e_{ref}(\tau) e^{k\tau} d\tau = \\ &= e^{kt} e_{ref}(t) - e^{kt_r^+} e_{ref}(t_r^+) - k \int_{t_r^+}^t e_{ref}(\tau) e^{k\tau} d\tau. \end{aligned} \quad (S15)$$

The obtained solution is substituted into the equation to calculate  $\mu_f(t)$ , and the first equation in (S3) is also considered:

$$\begin{aligned} \mu_f(t) &= e^{-k(t-t_r^+)} \mu_f(t_r^+) + e_{ref}(t) - e^{-k(t-t_r^+)} e_{ref}(t_r^+) - e^{-kt} k \int_{t_r^+}^t e_{ref}(\tau) e^{k\tau} d\tau = \\ &= e^{-k(t-t_r^+)} (\mu_f(t_r^+) - e_{ref}(t_r^+) + k e_f(t_r^+)) + e_{ref}(t) - k e_f(t) \end{aligned} \quad (S16)$$

The equation (S16) is substituted into the definition of  $\Delta_f(t)$  from (S6), as well as the equation (S5) and the initial conditions from (10)-(12) in the manuscript:

$$\begin{aligned}\Delta_f(t) &= B^\dagger (\mu_f(t) - \mu_{fd}(t)) = \\ &= B^\dagger \left( e^{-k(t-t_r^+)} (\mu_f(t_r^+) - e_{ref}(t_r^+) + k e_f(t_r^+)) + e_{ref}(t) - k e_f(t) - A_{ref} e_f(t) + B u_{adf}(t) \right) = \\ &= B^\dagger \left( e_{ref}(t) - k e_f(t) - e^{-k(t-t_r^+)} e_{ref}(t_r^+) - A_{ref} e_f(t) + B u_{adf}(t) \right)\end{aligned}\quad (S17)$$

The combination of (S14) and (S17) completes the proof of Lemma 1. □

## II. PROOF OF LEMMA 2 IN THE MANUSCRIPT

**Lemma 2.** *Let  $l > 0$  be sufficiently large, then the mixed regression is obtained as follows:*

$$Y(t) = \text{adj} \{ \varphi(t) \} y(t) = \det \{ \varphi(t) \} I_{p \times p} \Theta = \omega(t) \Theta. \quad (S18)$$

*Proof.* The equation (13) in the manuscript is substituted into the solution of the first equation from (14) in the manuscript:

$$y(t) = e^{-l(t-t_r^+)} y(t_r^+) + e^{-lt} \int_{t_r^+}^t e^{l\tau} \Phi_f(x(\tau)) \Phi_f^T(x(\tau)) \Theta(\tau) d\tau = e^{-lt} \int_{t_r^+}^t e^{l\tau} \Phi_f(x(\tau)) \Phi_f^T(x(\tau)) \Theta(\tau) d\tau. \quad (S19)$$

As the commutativity property with respect to  $\Theta^T(t)$  does not hold for the integral in (S7), then the right-hand side of (S19) is added and subtracted with  $\varphi(t) \Theta(t)$ :

$$y(t) = \varphi(t) \Theta(t) + \underbrace{e^{-lt} \int_{t_r^+}^t e^{l\tau} \Phi_f(x(\tau)) \Phi_f^T(x(\tau)) \Theta(\tau) d\tau - \varphi(t) \Theta(t)}_{\epsilon_1(t)}. \quad (S20)$$

The error  $\epsilon_1(t)$  is represented in the state space:

$$\begin{aligned}\epsilon_1(t) &= \chi_1(t) - \varphi(t) \Theta(t), \quad \epsilon_1(t_r^+) = 0_m, \\ \dot{\chi}_1(t) &= -l \chi_1(t) + \Phi_f(x(t)) \Phi_f^T(x(t)) \Theta(t), \quad \chi_1(t_r^+) = 0_m.\end{aligned}\quad (S21)$$

Taking into consideration (4), (12) in the manuscript and (S21), the error  $\epsilon_1(t)$  is differentiated:

$$\begin{aligned}\dot{\epsilon}_1(t) &= \dot{\chi}_1(t) - \dot{\varphi}(t) \Theta(t) - \varphi(t) \dot{\Theta}(t) = -l \chi_1(t) + \Phi_f(x(t)) \Phi_f^T(x(t)) \Theta(t) + l \varphi(t) \Theta(t) - \\ &- \Phi_f(x(t)) \Phi_f^T(x(t)) \Theta(t) - \varphi(t) \dot{\Theta}(t) = -l \epsilon_1(t) - \varphi(t) \dot{\Theta}(t) = -l \epsilon_1(t) - \varphi(t) \sum_j \theta_j \delta(t - t_j),\end{aligned}\quad (S22)$$

According to the properties of the delta-function, the solution of (S22) is written as:

$$\epsilon_1(t) = e^{-l(t-t_r^+)} \epsilon_1(t_r^+) + e^{-lt} \int_{t_r^+}^t e^{l\tau} \varphi(\tau) \sum_j \theta_j \delta(\tau - t_j) d\tau = e^{-l(t-t_r^+)} \epsilon_1(t_r^+) + e^{-lt} \sum_j e^{lt_j} \varphi(t_j) \theta_j h(t - t_j). \quad (S23)$$

As  $\epsilon_1(t_r^+) = 0_m$ , then the following piecewise definition is obtained on the basis of (S23):

$$\epsilon_1(t) = \begin{cases} 0_m, & \forall t \in [t_r^+; t_j) \\ e^{-lt} \sum_j e^{lt_j} \varphi(t_j) \theta_j h(t - t_j), & \forall t \geq t_j \end{cases}. \quad (S24)$$

or, if we consider the definition of  $t_r^+$ , then:

$$\epsilon_1(t) = \begin{cases} 0_m, & \forall t \in [t_k; t_j) \\ e^{-lt} \sum_j e^{lt_j} \varphi(t_j) \theta_j h(t - t_j), & \forall t \in [t_j; t_{k+1}) \end{cases}. \quad (S25)$$

Whence it follows that, if  $l > 0$  is chosen to be sufficiently large, then the equation  $\epsilon_1(t) = o(\varphi(t) \Theta(t))$  holds almost everywhere. As a result, the equation (S20) is rewritten without  $\epsilon_1(t)$ :

$$y(t) = \varphi(t) \Theta(t). \quad (S26)$$

The equation (S26) is multiplied by  $\text{adj} \{ \varphi(t) \}$  and the following property is applied:  $\forall A \in R^{n \times n} \text{adj} \{ A \} A = \det \{ A \} I_{n \times n}$ . As a result, the equation (S18) is obtained, which completes the proof of Lemma 2. □

### III. PROOF OF PROPOSITION 3 IN THE MANUSCRIPT

**Proposition 3.** If  $\omega(t) \in \text{FE}$  over the interval  $[t_r^+; t_e]$ , then

- 1)  $\forall t \geq t_r^+ \Omega(t) \in L_\infty, \Omega(t) \geq 0$ ;
- 2)  $\forall t \geq t_e \Omega(t) > 0, \Omega_{LB} \leq \Omega(t) \leq \Omega_{UB}$ .

*Proof.* To prove the first point of the proposition the upper bound of the regressor  $\Omega(t)$  is obtained from (17) in the manuscript:

$$\Omega(t) = \int_{t_r^+}^t \exp\left(-\int_{t_r^+}^t \sigma d\tau_1\right) \omega^2(\tau) d\tau \leq \delta \int_{t_0}^t \exp\left(-\int_{t_r^+}^t \sigma d\tau_1\right) d\tau \leq \frac{\delta}{\sigma} = \Omega_{UB},$$

$$\delta = \text{esssup}_{t \geq t_0} |\omega^2(t)|.$$
(S27)

According to Definition 2 in the manuscript, if  $\omega(t) \in \text{FE}$ , then  $\omega(t) \in L_\infty$  and  $\delta < \infty$ . So,  $\forall t \geq t_r^+ \Omega(t) \in L_\infty$ . In accordance with (16) in the manuscript  $\hat{\Omega}(t) \geq 0$ , then  $\Omega(t) \geq 0 \forall t \geq t_r^+$ . The first point of the proposition is proved.

To prove the second point of the proposition, following Definition 1 in the manuscript, the condition of the finite excitation of the regressor  $\omega(t)$  over the interval  $[t_r^+; t_e]$  is written:

$$\int_{t_r^+}^{t_e} \omega^2(\tau) d\tau \geq \alpha.$$
(S28)

Then  $\forall t \geq t_e$  the following holds:

$$\int_{t_e}^t \omega^2(\tau) d\tau > 0.$$
(S29)

As  $\exp\left(-\int_{t_r^+}^t \sigma d\tau_1\right) > 0$ , so the fact that (S29) holds results in (S30) holds too.

$$\Omega(t) = \int_{t_e}^t \exp\left(-\int_{t_r^+}^t \sigma d\tau_1\right) \omega^2(\tau) d\tau > 0, \forall t \geq t_e.$$
(S30)

For further proof of the proposition, the left-hand side of the inequality (S27) is rewritten so as to divide the whole time axis into two intervals:

$$\Omega(t) = \int_{t_r^+}^{t_e} \exp\left(-\int_{t_r^+}^t \sigma d\tau_1\right) \omega^2(\tau) d\tau + \int_{t_e}^t \exp\left(-\int_{t_r^+}^t \sigma d\tau_1\right) \omega^2(\tau) d\tau.$$
(S31)

According to  $\omega(t) \in L_\infty$ , (S27) and owing to  $\Omega(t) \geq 0$ , the first integral in (S31) is bounded from above:

$$\Omega(t) = \int_{t_r^+}^{t_e} \exp\left(-\int_{t_r^+}^t \sigma d\tau_1\right) \omega^2(\tau) d\tau \leq \Omega(t_e) = \Omega_{LB},$$
(S32)

Then, owing to (S27) and (S32),  $\forall t \geq t_e$  the following inequality holds for the regressor  $\Omega(t)$ :

$$\Omega_{LB} \leq \Omega(t) \leq \Omega_{UB},$$
(S33)

The second point of the proposition is proved.  $\square$

### IV. PROOF OF PROPOSITION 4 IN THE MANUSCRIPT

**Proposition 4.** If  $\omega(t) \in \text{FE}$  over the interval  $[t_r^+; t_e]$ , then  $\forall t > t_r^+$  the adaptation gain  $\Gamma_2(t)$  is bounded so that the following inequality holds:  $\Gamma_{2\min} \leq \Gamma_2(t) \leq \Gamma_{2\max}$ .

*Proof.* The following equality is used to prove Proposition 4:

$$\frac{d}{dt} 1 = \frac{d}{dt} \left[ \Gamma_2^{-1}(t) \Gamma_2(t) \right] = \Gamma_2(t) \frac{d\Gamma_2^{-1}(t)}{dt} + \Gamma_2^{-1}(t) \frac{d\Gamma_2(t)}{dt} = 0.$$
(S34)

The law to adjust  $\Gamma_2(t)$  from (18) in the manuscript is substituted into (S34). The obtained differential equation is solved  $\forall t > t_r^+$ :

$$\Gamma_2^{-1}(t) = \Gamma_2^{-1}(t_r^+) e^{-\lambda_1 t} + \lambda_2 \int_{t_r^+}^t e^{-\lambda_1(t-\tau)} \Omega^2(\tau) d\tau.$$
(S35)

According to the proof of Proposition 3, if  $\omega(t) \in \text{FE}$  over the interval  $[t_r^+; t_e]$ , then  $\forall t > t_e$  the estimate of  $\Omega(t)$  (S33) holds. As a result, using the mean-value theorem,  $\forall t > t_r^+$  the upper bound of  $\Gamma_2^{-1}(t)$  is written as:

$$\Gamma_2^{-1}(t) \leq \Gamma_2^{-1}(t_r^+) + \lambda_2 \Omega_{UB}^2 \int_{t_r^+}^t e^{-\lambda_1(t-\tau)} d\tau = \max \left\{ \Gamma_2^{-1}(t_r^+), \lambda_2 \lambda_1^{-1} \Omega_{UB}^2 \right\}.$$
(S36)

Then the lower bound of  $\Gamma_2^{-1}(t)$  is to be obtained. As the first summand of (S35) is strictly decreasing  $\forall t > t_r^+$ , while the second one, owing to the properties of the function  $\Omega(t)$  proved in Proposition 3, is increasing  $\forall t > t_r^+$ , then the minimum of their sum (S35) is at the point, in which the sum of their derivatives is zero when  $t < \infty$ . Then  $\forall t > t_r^+$  the following lower bound holds:

$$\Gamma_2^{-1}(t) \geq \Gamma_2^{-1}(t_r^+) e^{-\lambda T_{extr}} + \alpha \int_{t_r^+}^{T_{extr}} e^{-\lambda(T_{extr}-\tau)} \Omega^2(\tau) d\tau \geq \Gamma_2^{-1}(t_r^+) e^{-\lambda T_{extr}}, \quad (S37)$$

where  $T_{extr} < \infty$  is an *a priori* unknown time instant, when the absolute values of the derivatives of summands of (S37) are equal.

Combining (S36) and (S37) and transforming the  $\Gamma_2^{-1}(t)$  inequalities into  $\Gamma_2(t)$  ones, the following is obtained:

$$\underbrace{\min \left\{ \Gamma_2(t_r^+), \alpha^{-1} \lambda \Omega_{UB}^{-2} \right\}}_{\Gamma_{2 \min}} \leq \Gamma_2(t) \leq \underbrace{\Gamma_2(t_r^+) e^{\lambda T_{extr}}}_{\Gamma_{2 \max}}, \quad (S38)$$

as was to be proved. □

## V. PROOF OF THEOREM 1 IN THE MANUSCRIPT

**Theorem 1.** *If  $t_j \leq t_r^+$  and  $\Phi(x) \in \text{FE}$ , then the augmented error  $\xi(t)$  is exponentially stable ( $\xi(t) \in \text{GES}$ ).*

*Proof.* When  $t_j \leq t_r^+$ , then, according to Assumption 1 in the manuscript,  $\forall t > t_r^+ \ h(t - t_j) = 0$ . As a result,  $\forall t > t_r^+$  the following equality holds:

$$\Theta = \Theta_0 + \sum_j \theta_j h(t - t_j) = \Theta_0 + \Theta_1. \quad (S39)$$

Considering (S39) and (15) in the manuscript, the equation (17) in the manuscript is rewritten as  $\Upsilon(t) = \Theta \Omega(t)$ , and the derivative (20) in the manuscript  $\forall t > t_r^+$  is also rewritten as:

$$\dot{V}(\xi) = -e_{ref}^T Q e_{ref} - 2 \text{tr} \left( \tilde{\Theta}^T \Gamma_1^{-1} \Gamma_2 \Omega^2 \tilde{\Theta} \right), \quad (S40)$$

In accordance with the results of Proposition 3 proof,  $\forall t \geq t_e \ 0 < \Omega_{LB} \leq \Omega(t)$ . Then  $\forall t \geq t_e$  the upper bound of the derivative (S40) takes the form:

$$\dot{V}(\xi) \leq -\lambda_{\min}(Q) \|e_{ref}\|^2 - 2\lambda_{\min}(\Gamma_1^{-1}) \Gamma_{2 \min} \Omega_{LB}^2 \|\tilde{\Theta}\|_F^2 = -\frac{\min\{\lambda_{\min}(Q), \eta\}}{\lambda_M} V(\xi), \ \eta = 2\lambda_{\min}(\Gamma_1^{-1}) \Gamma_{2 \min} \Omega_{LB}^2. \quad (S41)$$

Having solved this inequality and applied the comparison lemma [S1],  $\forall t \geq t_e$  the following equation is obtained.

$$\|\xi(t)\| \leq \sqrt{\frac{\lambda_M}{\lambda_m} e^{-\kappa_{\min}(t-t_e)} \|\xi(t_e)\|}; \quad \kappa_{\min} = \lambda_M^{-1} \min\{\lambda_{\min}(Q), \eta\}. \quad (S42)$$

So, according to Definition 2 in the manuscript,  $\xi(t) \in \text{GES}$ , which proves the theorem. □

## VI. PROOF OF THEOREM 2 IN THE MANUSCRIPT

**Theorem 2.** *If  $t_j \in (t_r^+; t_e)$  and  $\Phi(x) \in \text{FE}$ , then the augmented error  $\xi(t)$  is exponentially ultimately bounded ( $\xi(t) \in \text{EUB}$ ) with the ultimate bound  $R$ .*

*Proof.* When  $t_j \in (t_r^+; t_e)$ , the equations (17) in the manuscript is written as:

$$\begin{aligned} \Omega(t) &= \int_{t_r^+}^t e^{-\int_{t_r^+}^t \sigma d\tau_1} \omega^2(\tau) d\tau = \underbrace{\int_{t_r^+}^{t_j} e^{-\int_{t_r^+}^t \sigma d\tau_1} \omega^2(\tau) d\tau}_{\Omega_1} + \underbrace{\int_{t_j}^t e^{-\int_{t_r^+}^t \sigma d\tau_1} \omega^2(\tau) d\tau}_{\Omega_2}; \\ \Upsilon(t) &= \underbrace{\int_{t_r^+}^{t_j} e^{-\int_{t_r^+}^t \sigma d\tau_1} \omega(\tau) Y(\tau) d\tau}_{\Upsilon_1} + \underbrace{\int_{t_j}^t e^{-\int_{t_r^+}^t \sigma d\tau_1} \omega(\tau) Y(\tau) d\tau}_{\Upsilon_2}; \end{aligned} \quad (S43)$$

In this case, the uncertainty parameters, according to (4) in the manuscript, are defined as:

$$\Theta = \begin{cases} \Theta_0, \forall t \in [t_r^+; t_j) \\ \Theta_0 + \underbrace{\sum_j \theta_j h(t - t_j)}_{\Theta_1}, \forall t \geq t_j \end{cases}; \quad (S44)$$

Taking into account the definition of the parameter error in (8) in the manuscript, the equations (S43) and (S44) are combined to obtain the regression  $\forall t \geq t_j$ :

$$\Upsilon(t) = (\Omega_1(t) + \Omega_2(t))\Theta_0 + \Omega_2(t)\Theta_1 = \Omega(t)\Theta_0 + \Omega_2(t)\Theta_1 = \Omega(t)\left(\tilde{\Theta}(t) - \Theta_1 + \hat{\Theta}(t)\right) + \Omega_2(t)\Theta_1, \quad (\text{S45})$$

where  $\Omega_2(t)$  is the unmeasurable regressor,  $\Theta_1$  is the vector of the unknown parameters.

Then, considering the equation (S45), the derivative (20) in the manuscript  $\forall t > t_j$  is written as:

$$\dot{V}(\xi) = -e_{ref}^T Q e_{ref} - 2\text{tr}\left(\tilde{\Theta}^T \Gamma_1^{-1} \Gamma_2 \Omega\left(\Omega\tilde{\Theta} - \Omega_1\Theta_1\right)\right). \quad (\text{S46})$$

As  $t_j \in (t_r^+; t_e)$ , then  $\Omega_1(t) \in \text{FE}$  and, using the equation (S40),  $\Omega_1(t)$  takes its maximum value at time instant  $t_j$ :

$$\Omega_1(t) = \int_{t_r^+}^{t_j} e^{-\sigma\tau} \omega^2(\tau) d\tau \leq \Omega_1(t_j) = \Omega_{1UB}. \quad (\text{S47})$$

Considering (S47) and (S33), the upper bound of the derivative (S46) for  $\forall t \geq t_e$  is obtained as:

$$\begin{aligned} \dot{V}(\xi) &\leq -\lambda_{\min}(Q) \|e_{ref}\|^2 + \eta \left[ -\|\tilde{\Theta}\|_F^2 + \eta_1 \eta^{-1} \|\Theta_1\|_F \|\tilde{\Theta}\|_F \right] \\ \eta_1 &= 2\lambda_{\max}(\Gamma_1^{-1}) \Gamma_{2\max} \Omega_{1UB} \Omega_{UB} \end{aligned} \quad (\text{S48})$$

Applying the method of completing the square to the expression in brackets in the equation (S48) and using the inequality  $-a^2 + ab \leq -\frac{1}{2}a^2 + \frac{1}{2}b^2$ , the following is obtained:

$$\dot{V}(\xi) \leq -\lambda_{\min}(Q) \|e_{ref}\|^2 - 0.5\eta \|\tilde{\Theta}\|_F^2 + \underbrace{0.5\eta(\eta_1 \eta^{-1})^2 \|\Theta_1\|_F^2}_{\varepsilon} \leq 0.5\kappa_{\min} V(\xi) + \varepsilon. \quad (\text{S49})$$

Having solved this inequality and applied the comparison lemma,  $\forall t \geq t_e$  the following is obtained:

$$\|\xi(t)\| \leq \sqrt{\frac{\lambda_M}{\lambda_m} e^{-0.5\kappa_{\min}(t-t_e)} \|\xi(t_e)\|^2 + 2\lambda_m^{-1} \kappa_{\min}^{-1} \varepsilon}. \quad (\text{S50})$$

So, according to Definition 3 in the manuscript,  $\xi(t) \in \text{EUB}$  with the ultimate bound  $R = \sqrt{2\lambda_m^{-1} \kappa_{\min}^{-1} \varepsilon}$ , which proves the theorem.  $\square$

## VII. PROOF OF THEOREM 3 IN THE MANUSCRIPT

**Theorem 3.** If  $t_j \geq t_e$  and  $\Phi(x) \in \text{FE}$ , then the augmented error  $\xi(t)$  is exponentially ultimately bounded ( $\xi(t) \in \text{EUB}$ ) with ultimate bound  $R_1$ .

*Proof.* As  $\Phi(x) \in \text{FE}$  over the interval  $[t_r^+; t_e]$ , then, when  $t_j \geq t_e$ ,  $\Phi(x) \notin \text{FE}$ . So, according to Proposition 1 and 2 in the manuscript,  $\omega(t) \notin \text{FE}$ . In this case, following Definition 1 in the manuscript, there exist no such  $t_s \geq t_j$   $T > 0$  and  $\alpha > 0$ , that the following inequality holds:

$$\int_{t_s}^{t_s+T} \omega^2(\tau) d\tau \geq \alpha \quad (\text{S51})$$

The inequality (S51) does not hold only if  $\omega(t) \equiv 0 \forall t \geq t_s \geq t_j$ . So  $\Omega_2(t) \equiv 0$  in (S43), and  $\forall t \geq t_j$  the regression (S45) is rewritten as:

$$\Upsilon(t) = \Omega(t) \left( \tilde{\Theta}(t) - \Theta_1 + \hat{\Theta}(t) \right) \quad (\text{S52})$$

Considering (S52),  $\forall t > t_j$  the derivative (20) in the manuscript is as follows:

$$\begin{aligned} \dot{V}(\xi) &= -e_{ref}^T Q e_{ref} - 2\text{tr}\left(\tilde{\Theta}^T \Gamma_1^{-1} \Gamma_2 \Omega^2\left(\tilde{\Theta} - \Theta_1\right)\right) \leq -\lambda_{\min}(Q) \|e_{ref}\|^2 + \eta \left[ -\|\tilde{\Theta}\|_F^2 + \eta_2 \eta^{-1} \|\Theta_1\|_F \|\tilde{\Theta}\|_F \right], \\ \eta_2 &= 2\lambda_{\max}(\Gamma_1^{-1}) \Gamma_{2\max} \Omega_{UB}^2 \end{aligned} \quad (\text{S53})$$

Similarly to (S49), applying the method of completing the square to the expression in brackets in the equation (S53) and using the inequality  $-a^2 + ab \leq -\frac{1}{2}a^2 + \frac{1}{2}b^2$ , the following is obtained:

$$\begin{aligned} \dot{V}(\xi) &\leq -\lambda_{\min}(Q) \|e_{ref}\|^2 - 0.5\eta \|\tilde{\Theta}\|_F^2 + \underbrace{0.5\eta(\eta_2 \eta^{-1})^2 \|\Theta_1\|_F^2}_{\varepsilon_1} \\ &\leq 0.5\kappa_{\min} V(\xi) + \varepsilon_1. \end{aligned} \quad (\text{S54})$$

Having solved this inequality and applied the comparison lemma,  $\forall t > t_j$  we have:

$$\|\xi(t)\| \leq \sqrt{\frac{\lambda_M}{\lambda_m} e^{-0.5\kappa_{\min}(t-t_j)} \|\xi(t_j)\|^2 + 2\lambda_m^{-1} \kappa_{\min}^{-1} \varepsilon_1}. \quad (\text{S55})$$

So, according to Definition 3 in the manuscript,  $\xi(t) \in \text{EUB}$  with the ultimate bound  $R_1 = \sqrt{2\lambda_m^{-1} \kappa_{\min}^{-1} \varepsilon_1}$ , which proves the theorem.  $\square$

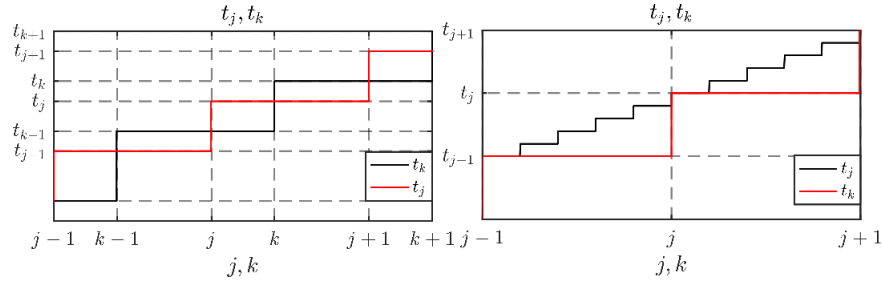

Fig. S1. Most preferable relationship between  $t_j$  and  $t_k$ .

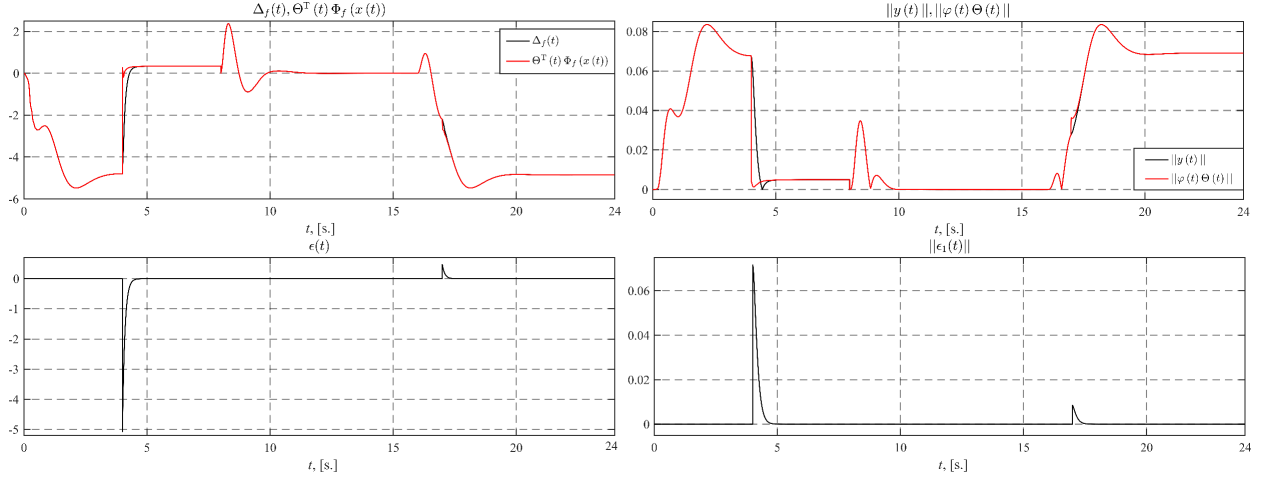

Fig. S2. Transient response of (a) functions  $\Delta_f(t)$  and  $\Theta^T(t) \Phi_f(x(t))$ , (b) disturbance  $\epsilon(t)$ , (c) functions  $\|y(t)\|$  and  $\|\varphi(t) \Theta(t)\|$ , (d) disturbance  $\|\epsilon_1(t)\|$ .

### VIII. MOST PREFERABLE RELATIONSHIP BETWEEN $t_j$ AND $t_k$

The piecewise-constant reference signal  $r(t)$  is used as an indicator of the time instant to reset the filters (11), (12), (14), (17) in the manuscript, which allows one to avoid superpositional integral-based mixing and ensure that only data of the current uncertainty (3) parameters are used in the adaptive law (18). So, the proposed adaptive control system provides the best possible performance when the following conditions hold for  $t_j$  and  $t_k$ :

$$\forall j, k \in \mathbb{N} \quad \begin{cases} \exists t_k \in [t_j; t_{j+1}), \\ t_{k+1} - t_k \ll t_{j+1} - t_j \end{cases} \quad (S56)$$

In other words, the conditions (S56) require to change the reference signal value more often than the uncertainty switches its parameters. If (S56) holds, then the number of intervals, in the course of which the error exponentially converges to zero, is maximized. Hence, the best quality of the reference trajectories (5) tracking is provided. If (S56) is not met, then, as proved in Theorems 2 and 3, the proposed closed-loop adaptive control system signals remain bounded, but the quality of the reference trajectories tracking reduces because the augmented error converges not to zero, but to a set with the bound  $R$  or  $R_1$ . Fig. S1 demonstrates the interrelations between  $t_j$  and  $t_k$ , which satisfy the conditions (S56).

Since in practice it is often impossible to ensure that (S56) is met, the problem to develop an algorithm to detect the uncertainty parameters (3) change and reset filters (11), (12), (14), (17) after such successful detection is actual (some preliminary results in this sense can be found in [S2]).

### IX. EXTENDED SIMULATION RESULT

The extended results of the numerical experiments are, firstly, to validate the conclusions made in Lemmas 1 and 2 with respect to disturbances  $\epsilon(t)$  and  $\epsilon_1(t)$ , and secondly, to demonstrate what influence the parameters  $l$  and  $k$  have on the transients quality of the augmented error.

Fig. S2 shows the transients of (a) functions  $\Delta_f(t)$  and  $\Theta^T(t) \Phi_f(x(t))$ , (b) disturbance  $\epsilon(t)$ , (c) functions  $\|y(t)\|$  and  $\|\varphi(t) \Theta(t)\|$ , (d) disturbance  $\|\epsilon_1(t)\|$ .

The obtained results prove the conclusions, which are made about the disturbances  $\epsilon(t)$  and  $\epsilon_1(t)$ : the piecewise definitions (S12) and (S24) hold,  $\epsilon(t)$  and  $\epsilon_1(t)$  converge exponentially to zero with the respective rate of  $l$  and  $k$ , which sufficiently large values ensure that  $\epsilon(t) = o(\Theta^T(t) \Phi_f(x(t)))$  and  $\epsilon_1(t) = o(\varphi(t) \Theta(t))$  hold almost everywhere.

Fig. S3 shows the transients of the augmented error  $\xi(t)$  norm for different values of the parameters  $l$  and  $k$ . The values of other parameters of the developed adaptive control system were the same for all experiments.

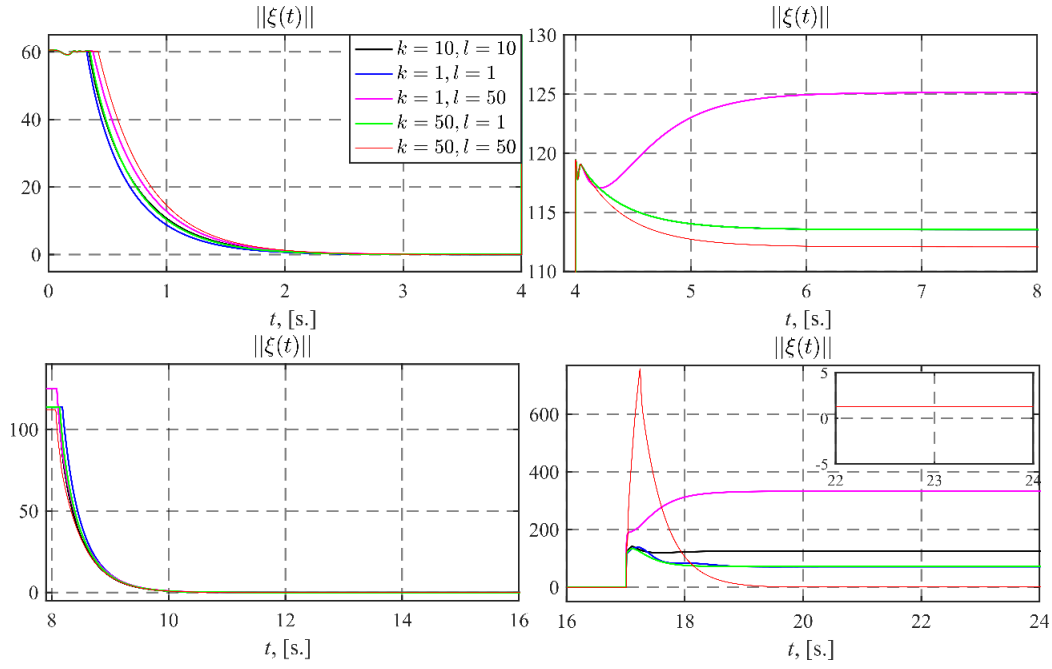

Fig. S3. Transient Response of  $\|\xi(t)\|$ .

Transients of  $\|\xi(t)\|$  demonstrate that the values of  $l$  and  $k$  affect the quality of transients over the time ranges  $[4; 8]$ ,  $[17; 24]$ , but not the exponential convergence of  $\|\xi(t)\|$  to zero over the intervals  $[0; 4]$ ,  $[8; 16]$ .

Thus, when the values of  $l$  and  $k$  are large, then the disturbances  $\epsilon(t)$  and  $\epsilon_1(t)$  decay quite fast, and the developed adaptive system provides the lowest value of the steady-state augmented error  $\xi(t)$ . However, in this case, significant peaks of  $\xi(t)$  may occur in the course of transients of the adjustable parameters  $\hat{\Theta}(t)$ . Therefore, according to the transients shown in Fig. S3, as far as the transients quality of the error  $\xi(t)$  is concerned, the best choice of the filter parameters (11), (12), and (14) is when the condition  $k \gg l$  is met.

## REFERENCES

- [S1] H. K. Khalil, *Nonlinear systems*, 3rd. New Jewsey, Prentice Hall, 9. 2002.
- [S2] A. Glushchenko, and K. Lastochkin, "Unknown Piecewise Constant Parameters Identification with Exponential Rate of Convergence," 2022. *Preprint*. Available: <https://arxiv.org/pdf/2203.11685.pdf>.
